# Supplementary material for: BDD100K: A Diverse Driving Dataset for Heterogeneous Multitask Learning
Source: arXiv:1805.04687 source file (2020-04-08)
Supplement: Supplementary file 1 [file mtl.tex]

We present more discussion for multitask learning in this section.
\subsection{Heterogeneous Multitask Learning}

For multitask learning experiment with BDD100K MOTS, we use the MOT model mentioned in Section 5.2 of the paper submission and add an mask head with four $3\times3$ convolution blocks and an $1\times1$ convolution to produce the segmentation outputs for each bounding box in the predicted track.
